# Supplementary material for: Automated Test Generation for Scratch Programs
Source: arXiv:2202.06274 source file (2022-08-23)
Supplement: Supplementary file 1 [file appendix.tex]

\section{Test Generation Algorithms}

\label{app:algorithms}

\begin{algorithm}
  \Input{\Scratch program $p$} 
  \Output{Test suite $T$}

  \Fn{\randomSearch{\( p \)}}{
    $G \gets$ coverage goals in \( p \)\tcp*{Set of all goals}
    $C \gets \emptyset$\tcp*{Set of already covered goals}
    $T \gets \emptyset$\tcp*{Test suite}
  
    \BlankLine
  
    \While{stopping condition not reached} {
      $\List{c_{1}, \ldots, c_{k}} \gets \generateRandomCodons(p)$\;
      \( t \gets \DecodeAndExecute(p, \List{c_{1}, \ldots, c_{k}}, \extractEvents) \)\;
      
      $C' \gets $ goals covered by \( t \)\;
      \If(\tcp*[f]{Check if \( t \) covers new goals}){$C' \minus C \neq \emptyset$}{
        $T \gets T \cup \{ t \}$\;
        $C \gets C \cup C'$
      }
    }
    
    \BlankLine
    
    \Return{$T$}\;
  }

  \BlankLine
  
  \Fn{\generateRandomCodons{p}}{
    \( \overline{C} \gets \List{} \)\;
    \( i \gets 0 \)\;
    \( k \gets \random(\{ 1, 2, \ldots \}) \)\;
    \While{\( i < k \)}{
      \( c \gets \random(\{ 0, 1, \ldots \}) \)\;
      \( \overline{C} \gets \overline{C} \plus \List{c} \)\;
      \( i \gets i + 1 \)\;
    }
    \Return{\( \overline{C} \)}\;
  }

  \caption{Random search}
  \label{alg:random_suite}
\end{algorithm}

\SetKwFunction{randomPopulation}{randomPopulation}
\SetKwFunction{updateArchive}{updateArchive}
\SetKwFunction{preferenceSorting}{preferenceSorting}
\SetKwFunction{sortByCrowdingDistance}{sortByCrowdingDistance}
\SetKwFunction{localSearch}{localSearch}

\SetKwFunction{DecodeAndExecuteAll}{decodeAndExecuteAll}

\begin{algorithm}
  \Input{program~\( p \) for which to generate tests}
  \Input{population size~\( N \in \mathbb{N} \)}
  \Output{test suite~\( A \) (an ``archive'' of test cases)}
	\Fn{\MOSA{\( p \), \( N \)}}{
   		$ P \gets \randomPopulation(p, N) $\;
      \( T \gets \DecodeAndExecuteAll(p, P) \)\;
       
    	$ A \gets \updateArchive(\emptyset, T) $\;
    	\While{stopping condition not satisfied} {
    		$ O \gets \textsf{generateOffspring}(P) $\;
        \( T \gets \DecodeAndExecuteAll(p, O) \)\;
	    	$ A \gets \updateArchive(A, T) $\;
	    	$ \List{F_{0}, F_{1}, F_{2}, \ldots} \gets \preferenceSorting(P \cup O) $\;
        $ P \gets \emptyset $\;
	    	$ i \gets 0 $\;
	    	\While{$ |P| + |F_i| \leq N $} {
				$ P \gets P \cup F_i $\;
				$ i \gets i + 1 $\;
			}
	    	$ \List{c_{1}, c_{2}, \ldots} \gets \sortByCrowdingDistance(F_i) $\;
        \( P \gets P \cup \{ c_{j} \mid j = 1, 2, \ldots, (N - |P|) \} \)\;
        \( (P, A) \gets \localSearch(P, A) \)\;
		}
  		\Return{$ A $}\;
  	}
    
    \BlankLine
    
    \Fn{\randomPopulation{\( p \), \( N \)}}{
      \( P \gets \emptyset \)\;
      \( i \gets 0 \)\;
      \While{\( i < N \)}{
        \( c \gets \generateRandomCodons(p) \)\;
        \( P \gets P \cup \{ c \} \)\;
      }
      \Return{\( P \)}\;
    }
    
    \BlankLine
    
    \Fn{\DecodeAndExecuteAll{\( p \), \( C \)}}{
      \( T \gets \emptyset \)\;
      \ForEach{codonSequence \( c \in C \)}{
        \( t \gets \DecodeAndExecute(p, c, \extractEvents) \)\;
        \( T \gets T \cup \{ t \} \)\;
      }
      \Return{\( T \)}\;
    }
    
    \caption{Many-Objective Sorting Algorithm~\citep{MOSA}}
    \label{alg:MOSA}
\end{algorithm}

\SetKwFunction{updateArchive}{updateArchive}
\SetKwFunction{random}{random}
\SetKwFunction{mutate}{mutate}
\SetKwFunction{getArchivePopulation}{getArchivePopulation}
\SetKwFunction{constructTestSuite}{constructTestSuite}
\SetKwFunction{chooseTarget}{chooseTarget}
\SetKwFunction{calculateDynamicParameter}{calculateDynamicParameter}
\SetKwArray{archive}{\ensuremath{\overline{A}}}

\begin{algorithm}
  \Input{program~\( p \)}
  \Input{set~\( K \) of targets in~\( p \)}
  \Input{start of the focused phase~\( F \in [0,1]\)}
  \Input{initial population size per target~\( n_0 \in \mathbb{N}\)}
  \Input{final population size per target~\( n_f \in \mathbb{N}\)}
  \Input{initial random selection probability~\( r_0 \in [0,1]\)}
  \Input{final random selection probability~\( r_f \in [0,1]\)}
  \Input{initial maximum mutation count~\( m_0 \in \mathbb{N}\)}
  \Input{final maximum mutation count~\( m_f \in \mathbb{N}\)}
  \Output{test suite~\( T \)}

	\Fn{\MIO{\( p \), \( K \), \( F \), \( n_0 \), \( n_f \), \( r_0 \), \( r_f \), \( m_0 \), \( m_f \)}}{
   		$ \archive \gets \emptyset^{|K|} $\;
   		$ B \gets $ depleted search budget\;
   		$ n \gets n_0$\;
   		$ r \gets r_0$\;
   		$ m \gets m_0$\;
   		\While{stopping condition not satisfied}{
   			\If {$B < F$}{
   				$ n \gets \calculateDynamicParameter(n_0, n_f, B, F)$\;
   				$ r \gets \calculateDynamicParameter(r_0, r_f, B, F)$\;
   				$ m \gets \calculateDynamicParameter(m_0, m_f, B, F)$\;
            }
   			\uIf{\( \archive = \emptyset^{|K|} \) or with probability~\( r \)} {
                $ \List{c_{1}, \ldots, c_{k}} \gets \generateRandomCodons(p) $\;
                \( t \gets \DecodeAndExecute(p,\List{c_{1}, \ldots, c_{k}}, \extractEvents) \)\;
                $ \archive \gets \updateArchive(\archive, t, n) $\;
                $ \archive \gets \localSearch(\{ t \}, \archive) $\;
            }
        \Else{
          $ k \gets \chooseTarget(K) $\;
          $ t \gets \random(A_k)$\;
          $ i \gets 0 $\;
          \While{$i < m$} {
            $ t' \gets \mutate(t) $\;
            $ \archive \gets \updateArchive(\archive, t', n) $\;
            \If {$t'$ has a better fitness value than $t$ for target $k$} 
            {
              $ t \gets t' $\;
            }
            $ i \gets i + 1 $\;
          }
          $ \archive \gets \localSearch(\{ t \}, \archive) $\;
        }
        $ B \gets $ updated search budget\;
	  }
	  $ T \gets \constructTestSuite(\archive, K)$\;
  	  \Return{$T$}\;
  	}
  	
  	\BlankLine
    
    \Fn{\calculateDynamicParameter{\( x_0 \), \( x_f \), \( B \), \( F \)}}{
    			\Return{$ x_0 + (x_f - x_0) \cdot \frac{B}{F} $}\;
    }
    
    \caption{Many Independent Objective Algorithm \citep{MIO}}
    \label{alg:MIO}
\end{algorithm}
